# Supplementary material for: DAdaQuant: Doubly-adaptive quantization for communication-efficient Federated Learning
Source: arXiv:2111.00465 ancillary file (2021-10-31)

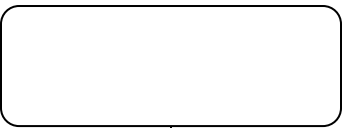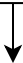

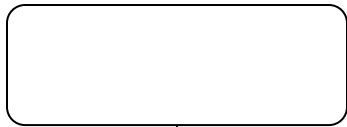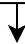

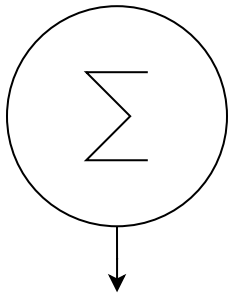



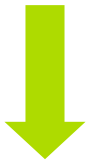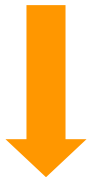

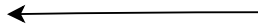







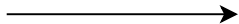

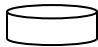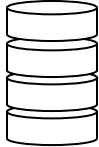

Supplement: Supplementary file 1 [file samplequant_complex_dynamic.pdf]
